# Supplementary material for: Adaptive Task Assignment in Online Learning Environments
Source: arXiv:1606.07233 source file (2016-06-23)
Supplement: Supplementary file 1 [file appendix.tex]

%\begin{appendices}

%\end{appendices}
